# Supplementary material for: Multimodal Large Language Models for Text-rich Image Understanding: A Comprehensive Review
Source: arXiv:2502.16586 source file (2025-02-23)
Supplement: Supplementary file 1 [file 7_Supp.tex]

\section{Datasets}

\subsection{Document}
Document understanding has evolved from early NLP tasks (summarization and plain text analysis) and perception tasks (layout analysis and key information extraction) to understanding and reasoning tasks in the current multimodal era. This evolution requires models not only to comprehend the meaning of text within visual images but also to possess certain computational capabilities, enabling them to answer questions ranging from ``Who is the author of this book'' (easy) to ``How many days until the medicine expires'' (hard). To enhance MLLMs with strong generalization abilities, many instruction tuning datasets have rapidly emerged, covering various document scenes such as receipts, bills, invoices, ID cards, forms, and more, in both single-page and multi-page VQA tasks. We provide a detailed introduction to important and widely used datasets, with additional datasets summarized in Table 1. 
For the single-page scenes, 

% provide an example
\noindent \textbf{DocVQA~\cite{mathew2021docvqa}} contains a mix of printed, typewritten and handwritten English content and focuses on letters, memos, notes, and reports. It includes a total of 12767 images with  50000 question-answer pairs. Among these QA pairs, the answers to questions are short text spans taken verbatim from the document, \emph{i.e.,} most of the answers can be retrieved from the given document images without the need for additional reasoning.

\noindent \textbf{Docmatix~\cite{laurenccon2024building}} leverages existing OCR tools to extract text from PDF documents and uses Phi-3-small to generate question-answer pairs. Low-quality question-answer pairs are filtered out using regular expressions, and answers containing the keyword "unanswerable" are removed. Ultimately, the dataset includes 2.4 million images and 9.5 million question-answer pairs derived from 1.3 million PDF documents. Compared to previous datasets, this represents a 240-fold increase in scale, significantly enhancing the scope of document understanding tasks.

\noindent \textbf{InfoVQA~\cite{mathew2022infographicvqa}} comprises a diverse collection of infographics annotated with question-answer pairs. It contains a total of 5,485 images and 30,035 question-answer pairs sourced from 2,594 different web domains. The questions in the dataset encompass table-based, graph-based, and visualization-based queries, as well as questions that require the integration of multiple cues. Given that most infographics include numerical data, the questions in the dataset also demand basic reasoning and arithmetic skills, such as counting, sorting, and performing arithmetic operations.

\noindent For the multi-page scenes,

\textbf{MP-DocVQA~\cite{tito2023hierarchical}} is designed for multi-page documents rather than single-page documents. It comprises 5,928 documents, 47,952 page images, and 46,176 question-answer pairs. These page images feature a diverse array of layouts, including tables, lists, charts, handwritten text, typed text, and printed fonts. The number of pages per document ranges from 1 to 20, providing a realistic scenario for multi-page document analysis.

\subsection{Chart}
Charts are essential visualization tools that assist users in analyzing data, extracting insights, and simplifying reading. Recently, with the advancement of AI systems, such as code generators, the method for collecting chart question-answer pairs has shifted from manual to automatic. For instance, by providing an appropriate prompt, GPT-4 can automatically generate chart rendering code, enabling the creation of chart images with the support of Python or MATLAB. From ChartQA to DVQA, the variety of chart types is expanding, and the complexity of question-answer tasks is increasing. We provide an in-depth introduction to key and widely utilized datasets, with additional datasets summarized in Table 1.

\noindent \textbf{ChartQA~\cite{masry2022chartqa}} focuses on answering questions about charts through visual and logical reasoning. This dataset includes human-authored complex reasoning questions that involve multiple logical and arithmetic operations, often referencing the visual features of the charts. It contains a total of 20,882 charts, with 9,608 human-authored questions and 23,111 automatically generated questions based on human-written chart summaries.

\noindent \textbf{PlotQA~\cite{methani2020plotqa}} consists of charts generated from real-world data sources, with questions generated based on crowdsourced question templates. The dataset includes a total of 224,377 charts and 28.9 million question-answer pairs. The questions cover three main categories: structural understanding, data retrieval, and reasoning, encompassing complex logical and numerical reasoning tasks.

\noindent \textbf{FigureQA~\cite{kahou2017figureqa}} is a dataset designed for visual reasoning, containing over one million question-answer pairs based on more than 100,000 synthetically generated scientific-style images. The images encompass five types of charts: line plots, dot-line plots, vertical and horizontal bar charts, and pie charts. The questions involve references to multiple chart elements and the integrated processing of spatial information. All answers to the questions are binary, being either Yes or No.

\noindent \textbf{DVQA~\cite{kafle2018dvqa}} is a dataset for data visualization question answering, focusing on understanding bar charts through a visual question answering framework. DVQA tests multiple aspects of bar chart comprehension, requiring the handling of words and answers unique to specific bar charts. It includes 300,000 charts and 3,487,194 question-answer pairs. The question types are: (1) Structural Understanding\textemdash Tests the system’s comprehension of the overall structure of the bar chart. (2) Data Retrieval\textemdash Assesses the system’s ability to retrieve information from the bar chart. (3) Reasoning\textemdash Evaluates the system’s capability to gather and manipulate information from multiple chart components. The answer types can be chart-specific text labels or numerical values.

\subsection{Natural Scene} 
Natural scenes are typically complex and variable, potentially including different lighting conditions, occlusions, and diverse object arrangements, which pose challenges to the robustness of MLLMs. For example, in a street scene image, the model should understand textual information (\emph{e.g.}, road signs and text on billboards) present in the images and integrate it with visual content to answer questions related to the images.

The types of VQA datasets are typically collected from two sources:

\noindent 1) Existing text datasets, such as TotalText, CTW1500, OPENVIVO, ICDAR-series datasets, etc.

\noindent 2) Subset selected from large-scale general natural scene images (\emph{e.g.}, LAION-5B, WuKong, COCO) based on the recognition results from an additional OCR engine.

In the following, we will introduce an in-depth analysis to 
 widely utilized datasets, with additional datasets summarized in Table 1.

\noindent \textbf{TextCaps~\cite{sidorov2020textcaps}} is a dataset for image captioning and reading comprehension, designed to assist visually impaired individuals in quickly understanding image content. The dataset comprises 28,408 images and 125,040 captions, requiring models to recognize text within images and relate it to the visual context to generate coherent descriptions. Unlike datasets organized in question-answer pairs, TextCaps facilitates the understanding and expression of image content through descriptive narratives.

\noindent \textbf{TextVQA~\cite{singh2019towards}} focuses on answering questions by reading and reasoning about text within images. The dataset includes 28,408 images and 45,336 question-answer pairs. These questions require models to recognize text in the images and perform reasoning within the context of both the image and the question to generate answers. The questions involve reading text in images and reasoning about it, including recognizing text content and understanding the relationship between the text and the image. Answers can be text directly extracted from the image or results derived from reasoning about the image and text.

\noindent \textbf{ST-VQA~\cite{biten2019scene}} focuses on leveraging textual information within images to answer questions. It comprises 23,038 images and 31,791 question-answer pairs. The questions require models to read text in the images and perform reasoning within the visual context to generate answers. Answers can be text directly extracted from the image or results derived from reasoning about the image and text. This dataset aims to emphasize the importance of utilizing high-level semantic information present in images during the visual question answering process.

% \noindent \textbf{OCR-VQA:}

\noindent \textbf{MT-VQA~\cite{wen2024mt}} is a dataset designed for multilingual text-centric visual question answering, aiming to address the challenges of visual text understanding in multilingual environments. It includes 8,794 images and 28,607 question-answer pairs. The dataset features high-quality human expert annotations in nine different languages, including Arabic (AR), Korean (KO), Japanese (JA), Thai (TH), Vietnamese (VI), Russian (RU), French (FR), German (DE), and Italian (IT). It covers a variety of text-rich image scenes, providing a comprehensive resource for multilingual visual understanding tasks.

\subsection{Table}
Tables are crucial for organizing and presenting structured data, enabling users to efficiently analyze and interpret information. With the advancements in AI systems, the approach to handling table-based question-answering tasks has evolved significantly. Initially, tasks focused on simple data retrieval and interpretation; however, they have now progressed to more sophisticated reasoning and analytical challenges. For instance, models are required to extract and synthesize information from tables to answer straightforward questions like "What is the total revenue for the year?" as well as more complex inquiries such as "Identify trends in sales growth across different product categories over multiple quarters."
To enhance the generalization capabilities of MLLMs in table-related tasks, various instruction-tuning datasets have been developed. These datasets encompass a wide range of table scenarios, including financial statements, statistical data tables, and spreadsheets, addressing both single-table and multi-table question-answering tasks. We provide a detailed introduction to key and widely used datasets, with additional datasets summarized in Table 1.

\noindent \textbf{TableQA~\cite{sun2020tableqa}} is a large-scale cross-domain Chinese natural language to SQL dataset, specifically designed for generating table-aware SQL queries. It contains over 6,000 tables, 64,891 question-answer pairs, and 20,311 unique SQL queries. The questions require models to handle condition values expressed in various ways, and some questions are unanswerable, adding to the dataset's challenge. More than 30\% of the samples need to be resolved through entity linking, compared to 3\% in the WikiSQL dataset and 5\% in the Spider dataset. There are over 5,000 unanswerable questions in the dataset, requiring models to recognize and manage these effectively.

% \noindent \textbf{ST-VQA:}

% \noindent \textbf{OCR-VQA:}

\subsection{Math}
Mathematical problem solving has evolved significantly, transitioning from simple arithmetic and algebraic tasks to complex geometric reasoning and theorem application in today's educational and computational landscape.  This progression demands models that not only understand mathematical text and diagrams but also possess advanced reasoning capabilities to solve problems such as "Calculate the area of the shaded region" (moderate) or "Prove the given geometric theorem" (challenging).  To enhance the capabilities of MLLMs in mathematical reasoning, various datasets have been developed, focusing on different aspects of mathematical problem solving. We provide an in-depth introduction to key and widely utilized datasets, with additional datasets summarized in Table 1.

\noindent \textbf{GeoQA~\cite{chen2021geoqa}} is a dataset of mathematical geometry question answering, designed to tackle geometric problems requiring a comprehensive understanding of textual descriptions, visual diagrams, and theorem knowledge. It includes 5,010 images paired with geometric problems, along with annotated solutions. The dataset is sourced from real Chinese middle school mathematics exam questions. The problems require models to simultaneously comprehend text and diagrams and perform multi-step reasoning involving geometric theorems and formulas.

\noindent \textbf{GeoQA+~\cite{cao2022augmented}} is an enhanced dataset for solving geometric problems, featuring a wider range and higher difficulty of geometric questions. Building on the original GeoQA dataset, it adds 2,518 new problems, totaling 7,528 questions, and is further expanded to 12,054 questions through data augmentation methods. The data is sourced from online educational websites and is aimed at students from grades 6 to 12.

\subsection{GUI}
%guicourse, seeclick, webui, odyssey, android_in_the_wild,amex
Graphical User Interfaces (GUIs) are typically designed to be informative and actionable for users. With the development of MLLMs, GUI agents have gained considerable traction. Increasingly more works, such as the MobileAgent series, OmniParser, OS-ATLAS, UI-Hawk, ShowUI, and others, explore the objective of allowing the agent to complete operations independently based solely on user instructions. Additionally, some related GUI datasets have been proposed based on various usage scenarios, including mobile apps, web pages, and PCs. However, most datasets primarily focus on screen and UI-based understanding and are not particularly relevant to document understanding. In this section, we list some related datasets to describe these scenarios.

\noindent \textbf{ScreenQA~\cite{hsiao2022screenqa}} is a question-answering dataset designed for screen content understanding, focusing on evaluating screen reading comprehension through mobile app screenshots. It contains 35,352 unique screenshots and 85,984 question-answer pairs. Annotated on the existing RICO dataset, ScreenQA aims to bridge the gap between structural and component-level understanding and higher-level tasks such as navigation and task completion. The questions involve extracting information from screenshots and reasoning about it, including short answers (\emph{e.g.}, phrases), full sentence answers, supporting UI content, and their bounding boxes. Answers can be short phrases, complete sentences, lists of UI content, and the bounding boxes of these contents.

\noindent \textbf{Screen2Words~\cite{wang2021screen2words}} is a dataset and method designed for automatic summarization of mobile user interfaces (UI), aimed at generating concise textual descriptions to convey the essential content and functionality of mobile screens. It includes 22,417 unique Android UI screens and 112,085 textual summaries. The task involves extracting information from screenshots and generating language descriptions, covering aspects such as screen type, UI elements, and application type. The summaries are produced through multimodal understanding of the screen content, resulting in language descriptions that effectively communicate the screen's key features and functions.

\section{Benchmark}
\subsection{Document}
In recent years, benchmark tests for document understanding have emerged successively, aiming to evaluate the capabilities of different models in processing complex documents.

Current benchmarks in document understanding primarily focus on two categories of text datasets: single-page documents and multi-page documents. In the context of single-page document understanding, datasets such as DocVQA~\cite{mathew2021docvqa} and InfoVQA~\cite{mathew2022infographicvqa} provide standardized frameworks for evaluating models' ability to extract information from a solitary page. These datasets are dedicated to exploring the recognition and comprehension abilities of OCR-based models regarding various text, table, and image elements.

However, although significant progress has been made in terms of recognition accuracy with current single-page document benchmarks, models often face greater challenges in understanding multi-page documents. MMLONGBENCH-DOC~\cite{Ma2024NEURIPS_MMLongBench_Doc_Benchmarking} serves as a new benchmark that systematically evaluates long textual documents. This dataset comprises 1,082 human-annotated questions based on 135 long documents with an average length of 47.5 pages, providing scenarios for cross-page information retrieval and understanding. Specifically, the MMLONGBENCH-DOC~\cite{Ma2024NEURIPS_MMLongBench_Doc_Benchmarking} dataset not only includes the extraction of various text and image elements but also introduces questions that require cross-page understanding and sets up unanswerable questions to detect potential hallucinations in information generation.

The innovation of this benchmark lies in its provision of diverse document sources and complexities, emphasizing the reasoning abilities across different information sources—an aspect less addressed in traditional document understanding benchmarks. Research indicates that the best model achieves only 44.9\% F1 score on MMLONGBENCH-DOC, further validating the shortcomings of current models in the context of long document understanding tasks.

Through comparisons with existing document understanding benchmarks, it is evident that most current datasets have limitations in information density and document length, often failing to adequately assess models' cross-page reasoning and information integration capabilities. Future work should focus on developing more effective frameworks for long document understanding to advance OCR technology and related models.
\subsection{Chart}
In recent years, with the rapid development of Multimodal Large Language Models (MLLMs), chart understanding has gradually gained extensive attention as a key research area. Existing chart-related benchmarks exhibit certain limitations, such as evaluating only a limited number of common chart types (\emph{e.g.}, line charts, bar charts, and pie charts) and relying on specific annotations within the charts to assess the model's performance in answering questions. This approach renders models less effective in real-world applications when confronted with unannotated charts, as they often depend on Optical Character Recognition (OCR) technologies to obtain potential answers and fail to comprehend the visual logic of the charts.

For instance, ChartQA~\cite{masry2022chartqa} and PlotQA~\cite{methani2020plotqa} are currently widely utilized benchmark datasets that primarily focus on three commonly encountered chart types. They depend on detailed point annotations, allowing models to easily access candidate answers when generating responses. However, this methodology weakens models' performance when handling non-annotated charts, as these models struggle to leverage visual cues such as colors, legends, and coordinate systems to perform reasoning. Consequently, there is a pressing need for improved evaluation benchmarks that address these cognitive limitations.

To tackle these issues, the new benchmark, ChartBench~\cite{Xu2024ARXIV_ChartBench_A_Benchmark}, has emerged. ChartBench is built upon 42 types of charts and their corresponding question-answer pairs, designed with a comprehensive evaluation methodology for chart understanding, which includes 66,600 charts and 600,000 question-answer pairs. The innovation of this benchmark lies in its significant expansion of chart diversity while emphasizing the evaluation of performance on unannotated charts, which is crucial for assessing the reliability of MLLMs in practical applications.

ChartBench introduces an enhanced evaluation metric, Acc+, which requires models to accurately judge both positive and negative assertions simultaneously, thereby minimizing arbitrary guesses in chart comprehension. This approach effectively assesses the models' understanding of visual information, extending beyond simple data point recognition to include reasoning regarding the logic and patterns present in the charts, thus providing a more realistic reflection of the models' performance in real-world contexts.
\subsection{Table}
At the intersection of OCR and NLP, Table Understanding has emerged as an important and complex research area. To this end, several relevant benchmarks such as TableVQA-Bench~\cite{Kim2024ARXIV_TableVQA_Bench_A}, TableQA~\cite{sun2020tableqa}, and TabPedia~\cite{Zhao2024NEURIPS_TabPedia_Towards_Comprehensive} have been proposed to evaluate models’ capabilities and effectiveness in handling visual table tasks.

TableVQA-Bench serves as a significant benchmark that focuses on Table Visual Question Answering (Table VQA) tasks. This benchmark integrates image and question-answering data, emphasizing the importance of multimodal visual information in answering and analyzing table content. TableVQA-Bench establishes a standardized evaluation framework, designed to provide question-answer pairs for various types of tables (\emph{e.g.}, financial tables, scientific tables, etc.), enabling models to assess their ability to extract and reason about table content in a unified environment. The design of this benchmark particularly emphasizes the effective utilization of image content and table information to produce accurate answers, advancing the development of table-based visual understanding technologies.

Building on this foundation, TableQA further integrates multiple table-related tasks, including Table Detection (TD), Table Structure Recognition (TSR), Table Querying (TQ), and Table Question Answering (TQA). This framework effectively encapsulates all aspects required for table understanding and highlights the synergistic effects of the tasks. TableQA collects a variety of public datasets (such as PubTab1M, FinTabNet, etc.) to provide the model with ample training samples and evaluation standards. Particularly in the TQ task, TableQA explores the challenges of extracting table structure from original document images and offers a new data synthesis method to enhance the model's generalization ability and understanding of complex scenarios.

TabPedia is a novel large vision-language model proposed in recent years, designed to unify table understanding tasks through a concept synergy mechanism. This model introduces meditative tokens, allowing various visual information to collaborate seamlessly, thereby maximizing the complementary effects across tasks such as table detection, structure recognition, querying, and answering. TabPedia employs multiple visual encoders (such as Swin Transformer and ViT) to extract fine-grained visual features of tables, combined with large language models (LLMs) to generate accurate responses and explanations. This model not only addresses the intricate details within tables but also enables reasoning in a multimodal context.

To further assess its performance in real-world scenarios, TabPedia has established a new comprehensive table question answering benchmark, ComTQA~\cite{Zhao2024NEURIPS_TabPedia_Towards_Comprehensive}, which includes approximately 9,000 question-answer pairs. Compared with existing table question answering benchmarks, ComTQA significantly enhances task complexity, encompassing mathematical calculations and reasoning problems, thereby propelling research on problem-solving capabilities that are more realistic and challenging.
